# Supplementary material for: FEDformer: Frequency Enhanced Decomposed Transformer for Long-term Series Forecasting
Source: arXiv:2201.12740 source file (2022-06-16)
Supplement: Supplementary file 1 [file algorithm.tex]

\section{Algorithm}
\label{app:alg1}
In this section, the detailed algorithm procedures of FEDformer, FEB and FEA are provided. The inputs of the encoder are the past $I$ time steps $X_\en \in \R ^{I \times D}$. The decoder contains two inputs, which are the seasonal part $X_\des \in \R^{\frac{I}{2}+O \times D}$ and the trend part $X_\det \in \R^{\frac{I}{2}+O \times D}$. $X_\det$ and $X_\des$ consist of two parts: 1) the seasonal part and trend part of the latter half of the encoder's input, 2) the constant padded part. $X_\det$ and $X_\des$ are formalized as
\begin{equation}
\label{app:algo:fun_initial_method}
\begin{aligned}
X_\ens,X_\ent &= \text{MOEDecomp}(X_{\en \frac{I}{2}:I}),\\
X_\des &= \text{Concat}(X_\ens, X_0),\\ 
X_\det &= \text{Concat}(X_\ent, X_\mean).\\
\end{aligned}
\end{equation}
% Using the above discussed input initialization method, 
The detailed algorithm procedures of FEB is given in Algorithm \ref{app:algo:FEB} and FEA is given in Algorithm \ref{app:algo:FEA}. The FEB and FEA serve as two inner blocks of the FEDformer network, and the overall algorithm procedure of the proposed FEDformer is given in Algorithm \ref{app:algo:fedformer}.

% the algorithms of FEDformer is given in Algorithm \ref{app:algo:fedformer}. In the FEDformer procedure, FEB and FEA serve as two inner blocks of the network. The algorithm of FEB is given in Algorithm \ref{app:algo:FEB} and FEA is given in Algorithm \ref{app:algo:FEA}.

% \mathrm\de

% \begin{algorithm}[tb]
%   \caption{Bubble Sort}
%   \label{alg:example}
% \begin{algorithmic}
%   \STATE {\bfseries Input:} data $x_i$, size $m$ \COMMENT{afwefae}
%   \REPEAT
%   \STATE Initialize $noChange = true$. %\algorithmiccomment{fawefa}
%   \FOR{$i=1$ {\bfseries to} $m-1$}
%   \IF{$x_i > x_{i+1}$}
%   \STATE Swap $x_i$ and $x_{i+1}$
%   \STATE $noChange = false$
%   \ENDIF
%   \ENDFOR
%   \UNTIL{$noChange$ is $true$}
% \end{algorithmic}
% \end{algorithm}

% \section{Algorithm 2}
\begin{algorithm}[h]
  \caption{Frequency Enhanced Block (FEB) Procedure}
\begin{algorithmic}[1]
  \STATE {\bfseries Input:} Input: series $X \in \mathbb{R}^{L \times D}$. The randomly selected M modes are used in Frequency domain, $M << L$. $R$ is randomly generated complex parameters, $\R \in \mathbb{C}^{N,d_{model},d_{model}}$.
  
\STATE $q$ = MLP($X$)
\STATE $\tilde{Q}$ = Select(FFT($q$, dim=0), dim=0) %\algorithmiccomment{test comment}
\STATE $R=$torch.randn($N,d_{model},d_{model}$) %\Commet{test comment}
\STATE $\tilde{Y}$=Einsum(`md',`mde'$\rightarrow$`me', $\tilde{Q}$, $R$)
\STATE $Y$=Zeros([$N, D$])
\STATE $Y[:M,:]$=$\tilde{Y}$
\STATE RETURN IFFT($Y$)
\label{app:algo:FEB}
\end{algorithmic}
\end{algorithm}

% \section{Algorithm 3}
\begin{algorithm}[h]
  \caption{Frequency Enhanced Attention (FEA) Procedure}
\begin{algorithmic}[1]
  \STATE {\bfseries Input:} Input: series $X_\en \in \mathbb{R}^{L \times D}$, $X_\de \in \mathbb{R}^{L \times D}$. The randomly selected M modes are used, $M << L$.
\STATE $q$ = MLP($X_\de$)
\STATE $k$, $v$ = MLP($X_\en$), MLP($X_\en$)
\STATE $\tilde{Q}$ = Select(FFT($q$, dim=0), dim=0)
\STATE $\tilde{K}$ = Select(FFT($k$, dim=0), dim=0)
\STATE $\tilde{V}$ = Select(FFT($v$, dim=0), dim=0)
\STATE $\tilde{Y}$= $\sigma (\tilde{Q} \cdot \tilde{K}^\top) \cdot \tilde{V}$
\STATE $Y$=Zeros([$N, D$])
\STATE $Y[:M,:]$=$\tilde{Y}$
\STATE RETURN IFFT($Y$)
\label{app:algo:FEA}
\end{algorithmic}
\end{algorithm}

\begin{algorithm}[h]
   \caption{Overall FEDformer Procedure}
%   \label{alg:example}
\begin{algorithmic}[1]
   \STATE {\bfseries Input:} Input: Input past time series $X \in \R^{I \times d}$ ; Input Length $I$; Predict length $O$; Data dimension $d$; Hidden state
channel $d_{model}$; Encoder layers number $N$; Decoder layers number $M$; Moving average window size $k$. Technically, we set $d_{model}$ as 512, $N$ as 2, $M$ as 1, $k$ as 25.
\STATE $X_\ens$, $X_\ent$ = MOEDecomp($X_{\frac{I}{2}:I}$)
\STATE $X_0$, $X_\mean$ = Zeros([$O,d$]), Repeat(Mean($X_{\frac{I}{2}:I}$, dim=0), dim=0)
\STATE $X_\des$, $X_\det$ = Concat($X_\ens,X_0$), Concat($X_\ent,X_\mean$)
\STATE $X_\en^0$ = Embed($X$)
\FOR {$l$ in \{1,...,N\}}
    \STATE $S_\en^{l,1},\_$ = MOEDecomp(FEB($X_\en^{l-1}$)+$X_\en^{l-1}$)
    \STATE $S_\en^{l,2},\_$ = MOEDecomp(FeedForward($S_\en^{l,1}$)+$S_\en^{l,1}$)
    \STATE $X^l_\en=S^{l,2}_\en$
\ENDFOr
\STATE $X^0_\de$ = Embed($X_\des$),$T^0_\de=X_\det$
\For{$l$ in \{1,...,M\}}
\STATE $S_\de^{l,1},T_\de^{l,1}$ = MOEDecomp(FEB($X_\de^{l-1}$) + $X_\de^{l-1}$)
\STATE $S_\de^{l,2},T_\de^{l,2}$ = MOEDecomp(FEA($S_\de^{l,1}, X_\en^N$) + $S_\de^{l,1}$)
\STATE $S_\de^{l,3},T_\de^{l,3}$ = MOEDecomp(FeedForward($S_\de^{l,2}$) + $S_\de^{l,2}$)

\STATE $T_\de^{l} =T_\de^{l-1}+W_{l, 1} \cdot T_\de^{l, 1}+W_{l, 2} \cdot T_\de^{l, 2}+W_{l, 3} \cdot T_\de^{l, 3}$
\STATE $X^l_\de=S^{l,3}_\de$
\ENDFOR

\STATE $X_\pred = W \cdot X_\de^M + T_\de^M$
\STATE RETURN $X_{\pred, \frac{I}{2}:\frac{I}{2}+O}$
\end{algorithmic}
\label{app:algo:fedformer}
\end{algorithm}
