# Supplementary material for: FEDformer: Frequency Enhanced Decomposed Transformer for Long-term Series Forecasting
Source: arXiv:2201.12740 source file (2022-06-16)
Supplement: Supplementary file 2 [file fourier_low_rank_approximation.tex]

\section{Fourier Transform}

% \paragraph{Fourier Transform in efficient computing}
Thanks to the algorithm of fast Fourier transform, the computation complexity of Fourier transform is compressed from N2 to NlogN. The Fourier transform has the property that convolution in time domain is equivalent to multiplication in frequency domain. Thus the FFt can be used in the acceleration of convolutional networks\cite{DBLP:MathieuHL13_fft_in_covolution}. FFt can also be used in efficient computing of auto-correlation function, which is useful in numerous anomaly detection\cite{IEEE-Homayouni-Autocorrelation-LSTM-anomaly-detection} and build neural networks block \cite{Autoformer}.

% \paragraph{Performance Boosting}
FNO can be used as a inner block to do representation learning in frequency domain. Combined with other layers, a SOTA result can be achieved. Fourier Neural Operator is first introduced in solving partial differential equations (PDEs)\cite{Fourier-Neural-Operator,Multiwavelet-based-Operator-Learning}. The FNO is also used in computer vision tasks\cite{DBLP:Global-filter-FNO-in-cv}.
It also serve as a working horse to build the Wavelet Neural Operator(WNO), which is recently introduced in solving PEDs\cite{Multiwavelet-based-Operator-Learning}

\section{Low Rank Approximation}
Linformer\cite{DBLP:journals/corr/abs-2006-04768-linformer} used trainable linear projection to compress the sequence length and achieved O(n) complexity with theoretically proving the boundary of approximation error based on JL lemma.  Luna\cite{DBLP:journals/corr/LUNA} developed a nested linear structure with O(n) complexity. BIGBIRD\cite{DBLP:conf/nips/Zaheer/BIGBIRD} used a sparse attention (Random+Global+Window attention) and achieved O(1) complexity.
Nystroformer\cite{DBLP:conf/aaai/XiongZCTFLS21/Nystroformer} used the idea of Nystrom approximation for the attention matrix and achieved a O(n) complexity. 
H-transformer\cite{DBLP:conf/acl/H-transformer} used hierarchical matrix for a sparse approximation of attention matrix with O(n) complexity. Performer\cite{DBLP:conf/iclr/Choromanski/Performer} used a linear attention via positive orthogonal random features approach. To the best of our knowledge, our proposed method is the first to apply fast attention mechanism through frequency domain low rank approximated transformation for time series prediction.
