# Supplementary material for: FEDformer: Frequency Enhanced Decomposed Transformer for Long-term Series Forecasting
Source: arXiv:2201.12740 source file (2022-06-16)
Supplement: Supplementary file 3 [file full_bench_multi.tex]

\begin{table}[!htbp]
\begin{adjustwidth}{-1.5in}{-1in}
\begin{tabular}{c|c|cccccccccccccccccccc}
\toprule
\multicolumn{2}{c|}{Methods}&\multicolumn{2}{c|}{FNO}&\multicolumn{2}{c|}{WNO}&\multicolumn{2}{c|}{Autoformer}&\multicolumn{2}{c|}{Informer}&\multicolumn{2}{c|}{LogTrans}&\multicolumn{2}{c|}{Reformer}&\multicolumn{2}{c|}{LSTM}&\multicolumn{2}{c|}{TCN}\\
\midrule
\multicolumn{2}{c|}{Metric} & MSE  & MAE & MSE & MAE& MSE  & MAE& MSE  & MAE& MSE  & MAE& MSE  & MAE\\
\midrule
\multirow{5}{*}{\rotatebox{90}{$ETTm2$}} &96 & 0.203 & 0.287 &\textbf{0.204} &\textbf{0.298} &0.255  &0.339  &0.365  &0.453  &0.768  &0.642  &0.658  &0.619    \\
                        & 192 & 0.269 & 0.328 &\textbf{0.268}  &\textbf{0.335}  &0.281 &0.340 &0.533  &0.563  &0.989  &0.757  &1.078  &0.827    \\
                        & 336 & \textbf{0.325} & \textbf{0.366} & 0.359 &0.387 &0.339  &0.372  &1.363&0.887  &1.334  &0.872  &1.549  &0.972     \\
                        & 720 & \textbf{0.421} & \textbf{0.415} &0.576 &0.501 &0.422  &0.419  &3.379  &1.3388 & 3.048 &1.328  &2.631  &1.242      \\
\midrule
\multirow{5}{*}{\rotatebox{90}{$Electricity$}} &96  & 0.180 & &\textbf{0.186} &\textbf{0.303} &0.201  &0.317  &0.274  &0.368  &0.258  &0.357  &0.312  &0.402    \\
                        & 192 &\textbf{0.199} & & 0.209 &\textbf{0.325} &0.222  &0.334  &0.296 &0.386  &0.266 &0.368  &0.348  &0.433    \\
                        & 336 & 0.329& &\textbf{0.212} &\textbf{0.313} &0.231 &0.338 &0.300  &0.394  &0.280 &0.380  &0.350  & 0.433    \\
                        & 720 & \textbf{0.237} & &0.246 &\textbf{0.355} &0.254  &0.361  &0.373  &0.439 &0.283  &0.376  &0.340  &0.420     \\
\midrule
\multirow{5}{*}{\rotatebox{90}{$Exchange$}} &96  & 0.148 & 0.278 &\textbf{0.139} &\textbf{0.276} &0.197  &0.323  &0.847  &0.752  &0.968  &0.812  &1.065  &0.829    \\
                        & 192 & 0.271 & 0.380 &\textbf{0.256} &\textbf{0.369} &0.300  &0.369  &1.204   &0.895 &1.040  &0.851  &1.188  & 0.906   \\
                        & 336 & 0.460 & 0.500 &\textbf{0.395} &\textbf{0.464} &0.509  &0.524  &1.672  &1.036  &1.659  &1.081  &1.357  &0.976     \\
                        & 720 & 1.429 & &\textbf{1.016} &\textbf{0.768} &1.447  &0.941  &2.478  &1.310  &1.941  &1.127  &1.510  &1.016     \\
\midrule
\multirow{5}{*}{\rotatebox{90}{$Traffic$}} &96  &0.622& &\textbf{0.562} &\textbf{0.349} &0.613  &0.388  &0.719  &0.391  &0.684  &0.384  &0.732  &0.423    \\
                        & 192 &0.626& &\textbf{0.562} &\textbf{0.346} &0.616&0.382  &0.696 &0.379  &0.685  &0.390  &0.733  &0.420    \\
                        & 336 &0.630& &\textbf{0.570} &\textbf{0.323} &0.622  &0.337  &0.777  &0.420  &0.733  &0.408  &0.742  &0.420     \\
                        & 720 &0.649& &\textbf{0.596} &\textbf{0.368} &0.660  &0.408  &0.864  &0.472  &0.717  &0.396  &0.755  &0.423     \\
\midrule
\multirow{5}{*}{\rotatebox{90}{$Weather$}} & 96 &0.242& &\textbf{0.227}  &\textbf{0.304}  &0.266  &0.336  &0.300  &0.384  &0.458  &0.490  &0.689  &0.596    \\
                        & 192 &0.372& &\textbf{0.295}  &\textbf{0.363}  &0.307  &0.367  &0.598  &0.544  &0.658  &0.589  &0.752  &0.638    \\
                        & 336 &0.445& &0.398  &0.421  &\textbf{0.359}  &\textbf{0.395 }  &0.578  &0.523  &0.797  &0.652  &0.639  &0.596    \\
                        & 720 &0.541& &0.531  &0.536  &\textbf{0.419}  &\textbf{0.428 }  &1.059  &0.741  &0.869  &0.675  &1.130  &0.792    \\
\midrule
\multirow{5}{*}{\rotatebox{90}{$ILI$}} & 24 &3.228& &\textbf{2.504}  &\textbf{1.051}  &3.483 &1.287  &5.764  &1.677  &4.480  &1.444  &4.400 &1.382    \\
                        & 36 &2.693& &\textbf{2.431}  &\textbf{1.000}  &3.103  &1.148  &4.755  &1.467  &4.799  &1.467  &4.783  &1.448    \\
                        & 48 &2.595& &\textbf{2.324}  &\textbf{1.000}  &2.669  &1.085  &4.763  &1.469  &4.800  &1.468  &4.832  &1.465    \\
                        & 60 &2.859& &\textbf{2.545}  &\textbf{1.061}  &2.770  &1.125 &5.264  &1.564  &5.278  &1.560  &4.882  &1.483    \\
\bottomrule
\end{tabular}
\caption{multivariate long sequence time-series forecating results on six datasets.}
\end{adjustwidth}
\end{table}
