# Supplementary material for: FEDformer: Frequency Enhanced Decomposed Transformer for Long-term Series Forecasting
Source: arXiv:2201.12740 source file (2022-06-16)
Supplement: Supplementary file 4 [file time_memory.tex]

\subsection{Model size and inference time}We plot memory usage and training time in Figure~\ref{fig_mem_speed}. Our proposed models show the linear GPU time and memory complexity in forecasting horizon. FEDformer-w is relatively slow in practice due to its recursive design. Among all, FEDformer-f with 16 modes achieves the best efficiency with little loss in accuracy, despite the deployment of MOE.

\begin{figure}[h]
\setlength{\abovecaptionskip}{-5pt}
\setlength{\belowcaptionskip}{-10pt} 
\vskip -0.13in
\begin{minipage}{0.5\linewidth}
    \centering
    \setlength{\abovecaptionskip}{-5pt}
    \setlength{\belowcaptionskip}{-10pt}
    \includegraphics[width=\linewidth]{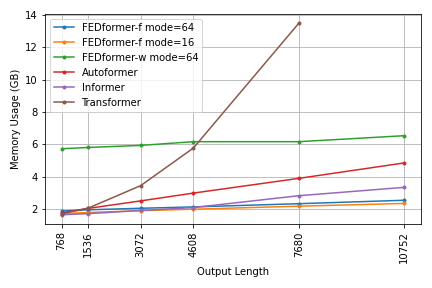}
    %\caption{Sample1:mean shift compared to input sequence}
    \end{minipage}\hfill
    \begin{minipage}{0.5\linewidth}
    \centering
    \setlength{\abovecaptionskip}{-5pt}
    \setlength{\belowcaptionskip}{-10pt}
    \includegraphics[width=\linewidth]{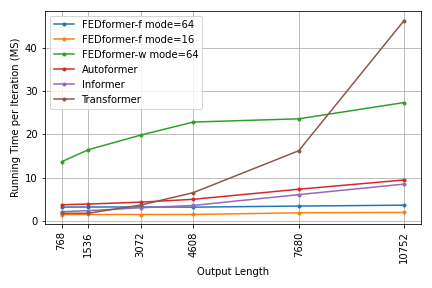}
    %\caption{Sample2:mean and frequency mode shifts compared to input sequence}
    \end{minipage}\hfill
    \vskip -0.15in
    \caption{Memory usage and training time comparison.}
    \label{fig_mem_speed}
    \vskip -0.25in
\end{figure} 
\vspace{-1mm}
