# Supplementary material for: FEDformer: Frequency Enhanced Decomposed Transformer for Long-term Series Forecasting
Source: arXiv:2201.12740 source file (2022-06-16)
Supplement: Supplementary file 5 [file univariate.tex]

\section{Univariate Results}
For the univariate prediction, FEDformer achieves the state-of-the-art performance in all six benchmarks. FEDformer yields a x\% relative reduction on MSE. To be specific: x\% in ETT, x\% in Electricity, x\% in Exchange, x\% in Traffic, x\% in Weather, x\% in ILI. 
\input{tables/tab_benchmark_s}
